# Supplementary material for: Selective Activation of Aromatic C-H Bonds Catalyzed by Single Gold Atoms at Room Temperature
Source: arXiv:2308.04658 source file (2023-08-09)
Supplement: Supplementary file 1 [file Au_DCA_Ag111_supporting_information_JACS_submission.pdf]

# Supporting Information: Selective Activation of Aromatic C-H Bonds Catalyzed by Single Gold Atoms at Room Temperature

Benjamin Lowe,[†,‡,⊥] Jack Hellerstedt,[†,‡,⊥] Adam Matěj,[¶,§,∥,⊥] Pingo Mutombo,[¶] Dhaneesh Kumar,[†,‡] Martin Ondráček,[¶] Pavel Jelinek,[*,¶,§] and Agustin Schiffrin[*,†,‡]

†*School of Physics and Astronomy, Monash University, Clayton, Victoria 3800, Australia*

‡*ARC Centre for Excellence in Low-Energy Electronics Technologies, Monash University, Clayton, Victoria 3800, Australia*

¶*Institute of Physics, Academy of Sciences of the Czech Republic, Cukrovarnická 10, 1862 53, Prague, Czech Republic*

§*Regional Centre of Advanced Technologies and Materials, Czech Advanced Technology and Research Institute (CATRIN), Palacký University Olomouc, 779 00 Olomouc, Czech Republic*

∥*Department of Physical Chemistry, Faculty of Science, Palacký University Olomouc, 771 46 Olomouc, Czech Republic*

⊥*Contributed equally to this work*

E-mail: jelinekp@fzu.cz; agustin.schiffrin@monash.edu

# Contents

**S1 Experimental methods** **S3**

S1.1 Sample preparation . . . . . . . . . . . . . . . . . . . . . . . . . . . . . . . . . . . . S3

S1.2 STM and STS measurements . . . . . . . . . . . . . . . . . . . . . . . . . . . . S3

S1.3 NcAFM measurements . . . . . . . . . . . . . . . . . . . . . . . . . . . . . . . . . S4

S1.4 STM lateral manipulation . . . . . . . . . . . . . . . . . . . . . . . . . . . . . . . S4

**S2 Theoretical methods** **S5**

S2.1 Gas-phase density functional theory (DFT) calculations . . . . . . . . . . . S5

S2.2 On-surface DFT calculations: electronic structure, total energy . . . . . . . S5

S2.3 Hybrid quantum mechanics/molecular mechanics (QM/MM) calculations . S6

S2.4 NcAFM simulations . . . . . . . . . . . . . . . . . . . . . . . . . . . . . . . . . . . S7

**S3 DCA+Au domains: structural characterization** **S7**

**S4 Structure of DCA-Au-DCA units: DFT** **S9**

**S5 NcAFM imaging simulations** **S9**

**S6 Electronic properties of DCA-Au-DCA dimers** **S10**

**S7 Au adatom character on Ag(111): DFT** **S12**

**S8 C-H bond dissociation energies: QM/MM calculations** **S14**

**S9 Orbital hybridization in reaction pathway** **S17**

**S10 Tentative pathway to organometallic dimers** **S25**

**S11 Second C-H bond activation** **S28**

**References** **S29**

# S1 Experimental methods

## S1.1 Sample preparation

The DCA+Au system was synthesized in UHV (base pressure $2 \times 10^{-10}$ mbar) by co-deposition of DCA molecules (Tokyo Chemical Industry; >95% purity) and Au (>99.99% purity) from the gas phase onto a clean Ag(111) surface held at room temperature (RT). The Ag(111) surface was cleaned by 2-3 cycles of sputtering with $Ar^+$ ions and subsequent annealing at ∼500°C. The DCA molecules (Au atoms, deposited simultaneously) were sublimated at 120°C (1040°C, respectively). The sample was held at RT for a further 1 hour before sample characterization. We also performed preparations with equivalent parameters in which DCA molecules then Au atoms were deposited sequentially. Both methods yielded qualitatively similar samples.

## S1.2 STM and STS measurements

All STM and d$I$/d$V$ STS measurements were performed at 4.5 K (base pressure $< 1 \times 10^{-10}$ mbar) with a hand-cut Pt/Ir tip. All STM images were acquired in constant-current mode with tunneling parameters as reported in the text (bias voltage applied to sample). All d$I$/d$V$ spectra were obtained by acquiring $I(V)$ as a function of bias voltage at a constant tip-sample distance (stabilized by a specified setpoint tunneling current and bias voltage), and by then numerically differentiating $I(V)$ to obtain d$I$/d$V$ as a function of bias voltage. All d$I$/d$V$ maps were acquired in constant-current mode (using setpoints $I_\mathrm{t} = 500$ pA and bias voltages as specified), with a lock-in technique by modulating the bias voltage with an amplitude of 10 mV at a frequency of 1.13 kHz, except the d$I$/d$V$ map in Figure S5b) (non-covalent DCA-only dimer) which was acquired via a single bias slice of the numerical derivative of pixel-by-pixel $I(V)$ curves.

## S1.3 NcAFM measurements

All ncAFM measurements were performed at 4.5 K in UHV (base pressure $< 1 \times 10^{-10}$ mbar) with a qPlus tuning fork sensor ($f_0 \approx 30$ kHz, $Q \approx 66$k, $K \approx 1.8$ kNm$^{-1}$, 50 pm amplitude modulation) with a CO-terminated Pt/Ir tip, in constant-height mode at a tip-sample distance defined by a STM setpoint (as specified in main text). The Pt/Ir tip was functionalized with a CO molecule by dosing CO gas into the UHV chamber ($5 \times 10^{8}$ mbar for 3 seconds) with the sample held at a temperature below 7 K. For functionalization, the tip was brought above a CO molecule adsorbed on Ag(111) at a height defined by the STM setpoint $V_{\mathrm{b}} = 20$ mV, $I_{\mathrm{t}} = 25$ pA. The tip was then lowered 375 pm to 'pick-up' the molecule before tunneling feedback was restored. Confirmation of symmetrical adsorption of CO at the tip apex was obtained by imaging other CO molecules on Ag(111) with the functionalized tip. CO molecules appearing in STM images as circular protrusions surrounded by an isotropic depression indicated successful symmetric CO-functionalization of the tip.

## S1.4 STM lateral manipulation

All lateral manipulation experiments were conducted with an Ag-terminated Pt/Ir STM tip at temperatures below 5 K. To remove individual DCA-Au-DCA dimers from the self-assembled DCA+Au domains, a tip-sample distance was defined by tunneling parameters $V_{\mathrm{B}} = -10$ mV, $I_{\mathrm{t}} = 14$ nA at a site in between DCA-Au-DCA dimers within the DCA+Au domain [start of blue arrow in main text Figure 2b)]. The tip was then translated laterally at a speed of 200 pm/s along paths specified in images. Once removed from the DCA+Au domain, we performed further lateral manipulation using a tip-sample distance defined by the tunneling parameters $V_{\mathrm{B}} = -10$ mV, $I_{\mathrm{t}} = 5$ nA above bare Ag(111) to move the DCA-Au-DCA units about the surface at the same tip speed.

# S2 Theoretical methods

## S2.1 Gas-phase density functional theory (DFT) calculations

Bond dissociation enthalpies (BDE), $\Delta H$, for gas phase DCA [Figure S7a)] were calculated by density functional theory (DFT) with the Gaussian16 package,[1] using the $\omega$B97X-D functional[2] with the def2-SVP basis set.[3]

We also carried out DFT calculations using the FHI-AIMS code[4] to investigate the electronic properties and total energy of certain DCA complexes in the gas phase. We performed these calculations at the B3LYP level,[5] using the Tkatchenko-Scheffler treatment of the van der Waals interactions.[6] This method was used for calculations shown in sections S6 and S9 below.

## S2.2 On-surface DFT calculations: electronic structure, total energy

We carried out DFT calculations using the FHI-AIMS code[4] to investigate the electronic properties and total energy of DCA and its complexes on both Ag(111) and Au(111) surfaces. We performed these calculations at the GGA-PBE[7] level, using the Tkatchenko-Scheffler treatment of the van der Waals interactions.[6] As Ag(111) and Au(111) surfaces, we employed a $5 \times 11$ supercell with three atomic layers (see SI Figure S6). All atoms of the supercell structure were structurally relaxed except for the bottom layer furthest from the adsorbates. Convergence was achieved when atomic force and total energy differences were below $10^{-2}$ eV/Å and $10^{-5}$ eV, respectively. We used a single $\Gamma$ point to sample the Brillouin zone.

## S2.3 Hybrid quantum mechanics/molecular mechanics (QM/MM) calculations

We employed quantum mechanics/molecular mechanics (QM/MM) simulations to calculate total energy differences, $\Delta E$, and Gibbs free energy differences, $\Delta G$, for different systems composed of DCA molecules and Au atoms adsorbed on Ag(111) (see main text Figure 5, and Figures S7, S8, S16), at $T = 0$ and 300 K. We used the umbrella sampling method to calculate $\Delta G$ along different reaction pathways. We employed Sander[8] as the main program with Fireball[9] as the code for QM calculations. The QM calculations with Fireball used the BLYP[5,10] exchange correlation functional with D3 corrections,[11] and a basis set consisting of optimized numerical atomic-like orbitals,[12] i.e., s orbital for H, $sp^3$ orbitals for C and N, and $sp^3d^5$ for Au and Ag. The accuracy of the QM/MM Fireball-Sander method has been previously benchmarked with QM/MM Gaussian-Sander simulations using B3LYP[5,13,14]/def2-SVP, validating the use of Fireball in these conditions.[15]

In main text Figure 5, the reaction coordinate for the umbrella sampling of $\Delta G$ was set along the C-H bond of interest for the systems in panels b) and c); for the system in panel d), the reaction coordinate was defined as the difference between the lengths of C-H and Au-H bonds involved in the reaction. For each reaction pathway, $\Delta G$ was calculated by: (i) starting from the transition state TS determined beforehand, the system was steered both towards the initial state IS as well as the intermediate state IM; at each frame the system was relaxed (structurally and electronically) via DFT with an applied restraint on the reaction coordinate (with $T = 0$ K); (ii) the system was then tempered from 0 to 300 K via a molecular dynamics (MD) simulations of 600 time steps of 0.5 fs; (iii) finally, a set of MD simulations was submitted for each frame with 5000 time steps of 0.5 fs. The $\Delta G$ profiles were obtained by collecting the restrained bond lengths at each step and via a weighted histogram analysis method.

### S2.4 NcAFM simulations

The simulations of the ncAFM images [main text Figure 3b); Figure S3) were based on the probe-particle model[16] which includes van der Waals (vdW) and electrostatic interactions between the CO tip and the surface. All simulations were performed with a charge scaling of $-1e$ at the probe apex and a probe lateral stiffness ($k$) of 0.25 N/m. The electrostatic forces were obtained based on the Hartree potential calculated from the total energy FHI-AIMS DFT calculations.

## S3 DCA+Au domains: structural characterization

Figure S1 shows STM and ncAFM topographic images of self-assembled DCA+Au domains with cis (a) and trans (b-e) DCA-Au-DCA units. We determined the registration of the DCA+Au domains with respect to the substrate by atomically resolved imaging of bare Ag(111) [top of Figure S1d), e); red circles indicate Ag atom positions] and by subsequently extrapolating the Ag(111) atomic lattice within the DCA+Au domains, showing the adsorption position of the DCA-Au-DCA units. The self-assembled DCA+Au domains are incommensurate with the Ag(111) surface, with unit cell vectors [$\mathbf{b}_1$, $\mathbf{b}_2$ in Figure S1b)] forming an angle of $5.0 \pm 0.5^{\circ}$ with respect to the Ag(111) unit cell vectors. The cis and trans domain configurations have equivalent lattice vectors, with $\mathbf{a_1}$ being $\sim$twice as long as $\mathbf{b_1}$ to account for the alternating orientations of the cis DCA-Au-DCA units. We also sporadically observed bright ncAFM features at the center of some of the DCA-Au-DCA units [indicated by dashed circles in Figure S1c)-e)]. We claim that these are likely adsorbed residual gas molecules. We tentatively suspect they may be CO molecules (deliberately introduced for ncAFM) based on observations of inadvertent tip functionalization during manipulation experiments.

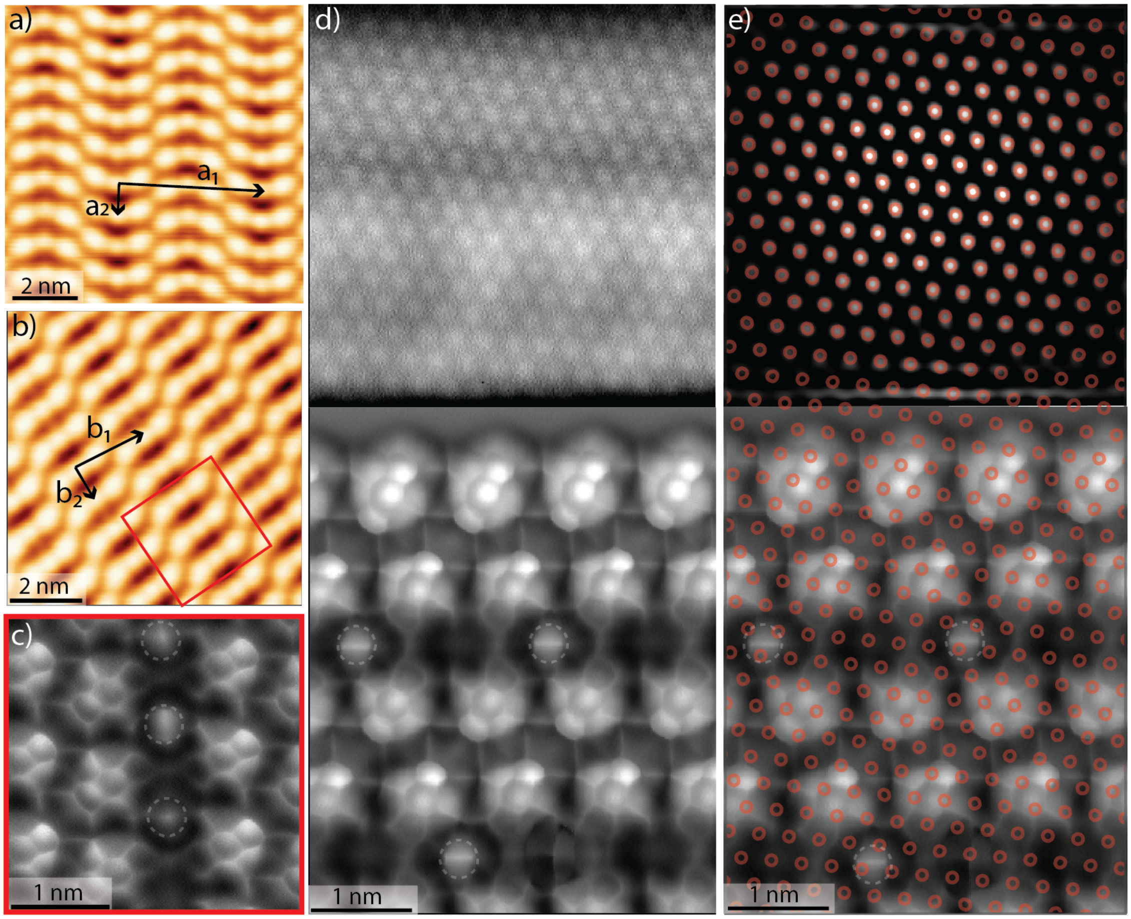


Figure S1: Organometallic DCA-Au-DCA dimers in self-assembled DCA+Au domains on Ag(111). a)-b) Constant-current STM images with cis ($I_t$ = 25 pA) and trans ($I_t$ = 10 pA) DCA-Au-DCA dimers, respectively ($V_b = -20$ mV). Vectors $\mathbf{a}_1$ and $\mathbf{a}_2$, and $\mathbf{b}_1$ and $\mathbf{b}_2$ define primitive unit cell vectors of the 2D domains ($a_1 = 4.38 \pm 0.05$ nm, $a_2 = 0.97 \pm 0.05$ nm, $b_1 = 2.08 \pm 0.05$ nm, $b_2 = 1.05 \pm 0.05$ nm). c) CO-tip constant-height ncAFM image of region of trans DCA+Au domain shown in the red box in b) (tip 30 pm closer to sample with respect to STM setpoint $V_b$ = 15 mV, $I_t$ = 100 pA). d)-e) CO-tip constant-height ncAFM image of trans DCA+Au domain boundary. Top: Atomically resolved bare Ag(111) area (tip height defined by STM setpoint $V_b$ = 3 mV, $I_t$ = 700 pA). Bottom: trans DCA-Au-DCA dimers (tip 30 pm closer to sample with respect to STM setpoint $V_b$ = 15 mV, $I_t$ = 100 pA). e) Same as d), with Fourier filtering of the bare Ag(111) region to emphasize the atomic lattice. Red circles indicate Ag atom positions [based on bare Ag(111) at the top] allowing us to determine the DCA+Au domain registration with respect to the substrate. Sporadic bright features at the center of some of the DCA-Au-DCA units in c)-e) (indicated by dashed circles) are likely adsorbed residual gas molecules.

# S4 Structure of DCA-Au-DCA units: DFT

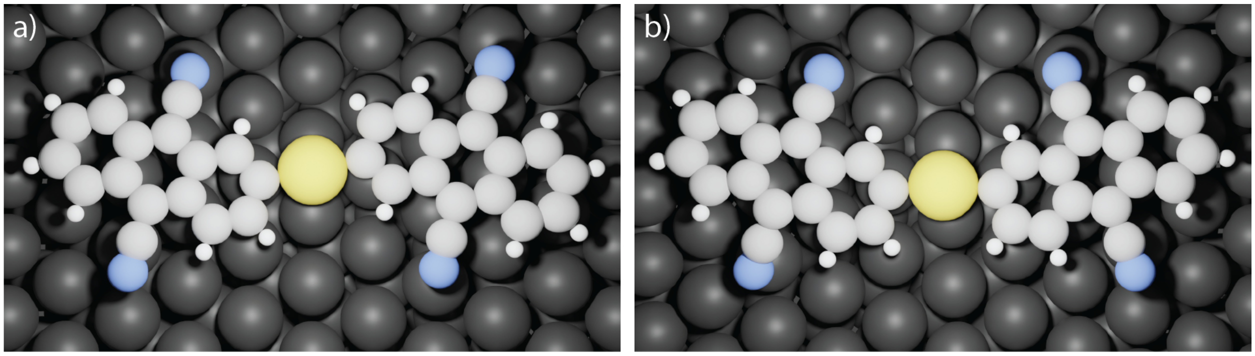


Figure S2: Ball-and-stick schematic of structure of DFT-relaxed trans (a) and cis (b) DCA-Au-DCA dimers on Ag(111) (see Section S2.2). The total energy difference between the two configurations is only ~0.2 kcal/mol which indicates that both are similarly stable, consistent with their observed coexistence in experiments.

# S5 NcAFM imaging simulations

Figure S3 shows a comparison between simulated and experimental ncAFM images of organometallic DCA-Au-DCA and organic DCA-DCA (i.e., covalently bonded via position A carbon atoms) units. The simulated ncAFM image for a DFT-relaxed DCA-Au-DCA dimer [Figure S3a)] shows good qualitative agreement with the experimental image [Figure S3g)], with a reduced frequency shift $\Delta f$ for the benzene rings closest to the Au atom (i.e., darker appearance) in comparison to the other DCA benzene rings, and the experimentally measured distance $d \approx 6.0$ Å between the centers of these benzene rings similar to $d \approx 5.72$ Å in the simulation. Importantly, the simulated ncAFM image of an hypothesized DCA-DCA dimer (with a covalent C-C bond between position A carbon atoms) fails to qualitatively capture such experimentally observed features, with a significantly larger $\Delta f$ at the DCA-DCA linkage and significantly smaller $d \approx 4.76$ Å. These findings support our claim that the experimentally observed Au-induced structure consist of an organometallic DCA-Au-DCA dimers featuring a covalent C-Au-C bonding motif. Since purely organic molecular domains were observed when only DCA molecules were deposited on Ag(111) (i.e., without Au de-

position),[17] we also claim that Ag atoms from the Ag(111) surface do not play a role in the formation of the DCA-Au-DCA dimer motif.

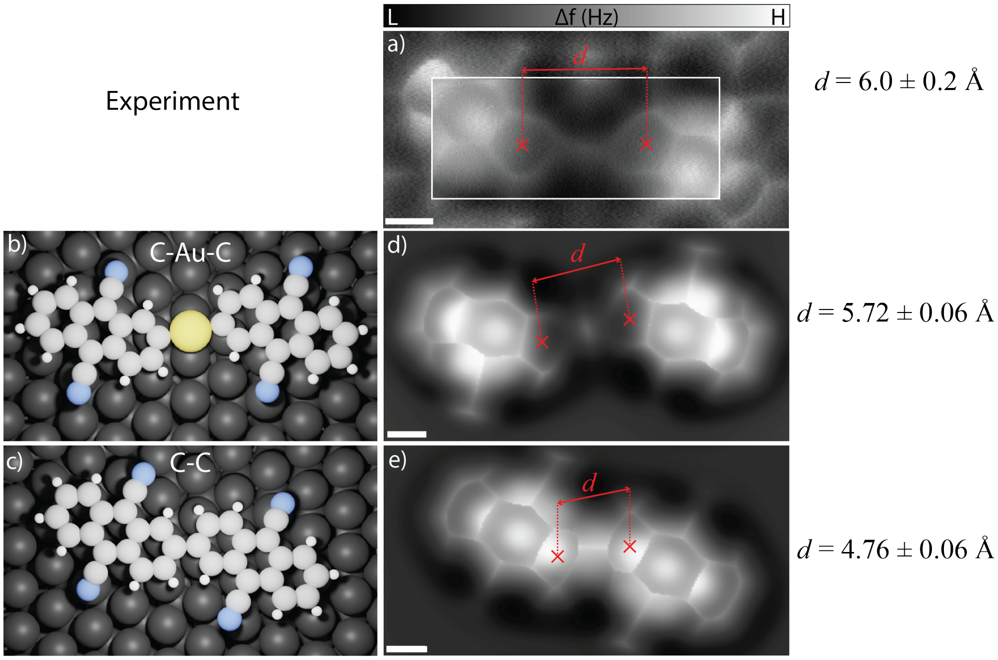


Figure S3: Comparison of experimental and simulated ncAFM images. a) Experimental constant-height ncAFM image of DCA-Au-DCA dimer, acquired with a CO-functionalized tip (tip 30 pm closer to sample with respect to STM setpoint $V_b = 15$ mV, $I_t = 100$ pA), showing good agreement with simulated ncAFM image in d), in particular regarding the distance $d$ between the centres of the two benzene rings closest to the Au atom. b), c) Ball-and-stick models of DFT structurally optimized DCA-Au-DCA and DCA-DCA dimers on Ag(111) (see Section S2.2). d), e) Probe-particle ncAFM simulations for structures in (b, c).

# S6 Electronic properties of DCA-Au-DCA dimers

Figure S4 shows the projected density of states (PDOS) of a gas-phase DCA-Au-DCA dimer as calculated by DFT (see Methods), with contributions from DCA and Au states (top), and specifically from Au 5d states (bottom). The calculated LUMO and LUMO+1 have predominantly DCA character, with a small contribution from the Au $5d_{yz}$ orbital, consistent with the experimental $dI/dV$ maps in Figure 4 of the main text. The spatial distribution of these states, both experimentally [Figure 4b), c) in main text] and theoretically [Figure 4e),

f) in main text], is similar to that of the previously observed DCA LUMO.[17]

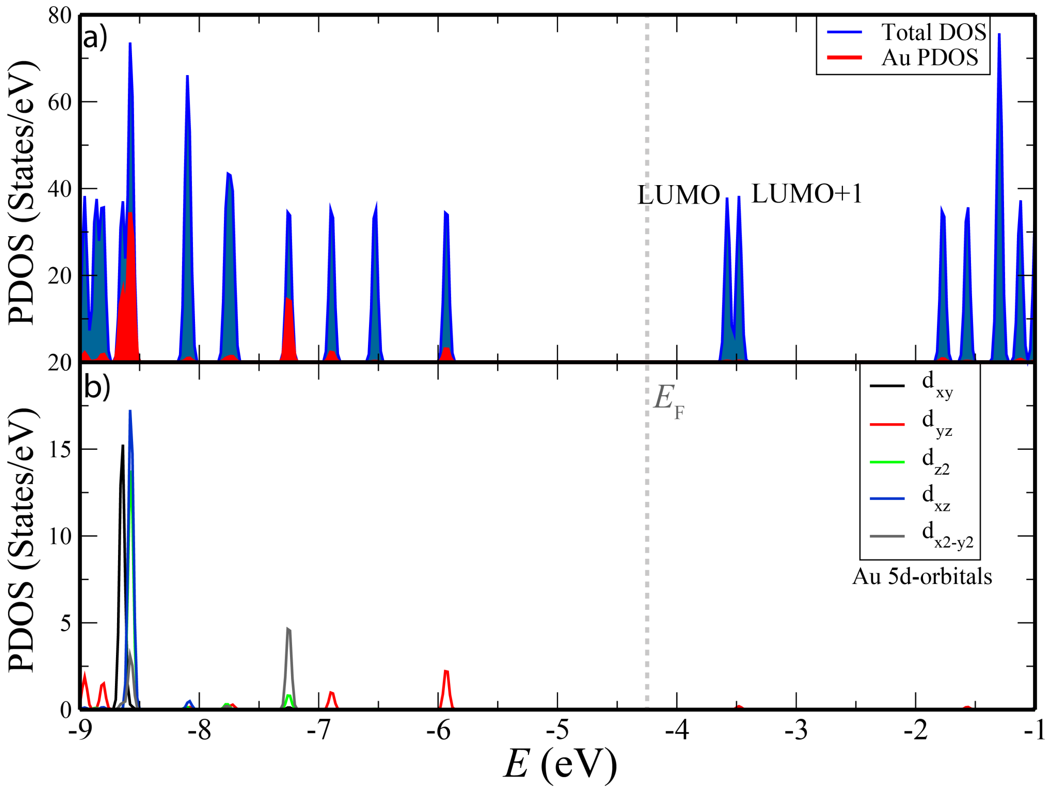


Figure S4: Projected density of states (PDOS) of gas-phase DCA-Au-DCA dimer calculated by DFT (B3LYP), as a function of energy. a) Total density of states (blue) and Au PDOS (red). b) PDOS onto Au 5d orbitals. Dashed grey line indicates position of Fermi level ($E_F$). This electronic structure calculation is related to Figure 4e-f) in main text.

Figure S5 shows d$I$/d$V$ spectra and maps for an organic, non-covalently bonded DCA-only dimer and for an organometallic DCA-Au-DCA dimer [data for the latter are the same as in main text Figure 4a-c)]. The d$I$/d$V$ spectrum taken at the anthracene end of the DCA-only dimer [red curve in Figure S5a)] shows a peak at $V_b \approx 0.47$ V attributed to the DCA LUMO, as observed previously.[17] In contrast, spectra for the organometallic DCA-Au-DCA dimer [blue and orange curves in Figure S5a), b)] show a peak at lower energy ($V_b \approx 0.38$ V) and a peak at higher energy ($V_b \approx 0.56$ V), that we attribute to the LUMO and LUMO+1 of the DCA-Au-DCA system (see main text). Based on this and on the predominantly molecular character of these LUMO and LUMO+1 determined via DFT (Figure S4), we

claim that these molecular states of the DCA-Au-DCA dimer are the result of hybridization between the two DCA LUMOs mediated by the DCA-Au covalent bonding.

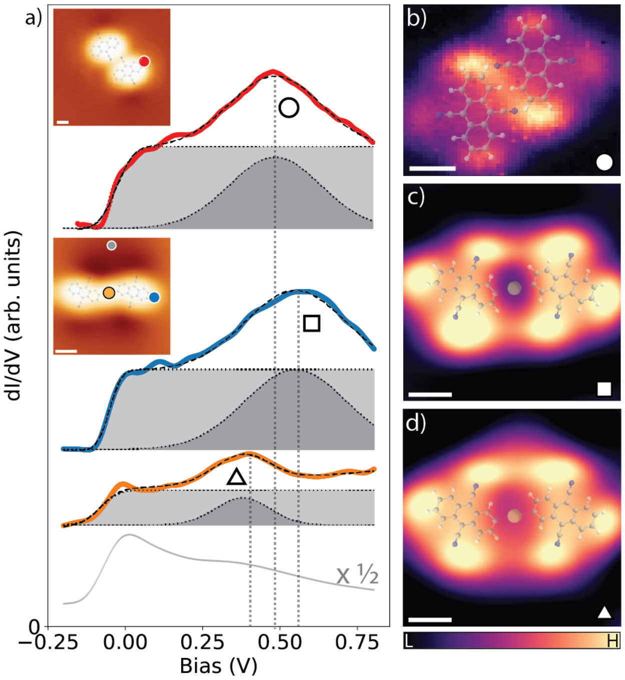


Figure S5: Electronic properties of organic DCA-only dimer and organometallic DCA-Au-DCA dimer on Ag(111). a) $dI/dV$ spectra for DCA-only dimer (red), DCA-Au-DCA dimer (blue, orange) and bare Ag(111) (gray), acquired at sites indicated in insets. Setpoints: $V_b$ = -200 mV, $I_t$ = 20 pA [DCA-Au-DCA; Ag(111)]; $V_b$ = -200 mV, $I_t$ = 10 pA (DCA-only; see Methods). Curves offset for clarity. Grey shaded regions are fits (error function plus Gaussian peak) of experimental data. Insets: constant-current STM images of DCA-only (top) and DCA-Au-DCA (bottom) dimers ($V_b$ = -20 mV, $I_t$ = 50 pA). b) Slice of pixel-by-pixel $dI/dV$ curves obtained via the numerical derivative of $I(V)$ curves (setpoint $V_b$ = -200 mV, $I_t$ = 1 pA) at a bias of 486 mV. c) - d) $dI/dV$ maps (constant current $I_t$ = 500 pA) at 400 and 550 mV, respectively, for an organometallic DCA-Au-DCA structure (constant-current lock-in method). All scale bars: 5 Å.

# S7 Au adatom character on Ag(111): DFT

Figure S6a) shows the density of states (PDOS), projected onto Au 5d states, of an Au adatom on Ag(111) and on Au(111), as a function of energy. This PDOS was calculated via DFT at the B3LYP level (see Method). The PDOS for Au on Ag(111) is a lot sharper than on Au(111). The energy broadening of the adatom Au 5d states on Au(111) is indicative of

significant electronic hybridization between adatom and surface, while the sharp PDOS on Ag(111) shows that the electronic character of Au on Ag(111) is close to that of an isolated neutral Au atom.

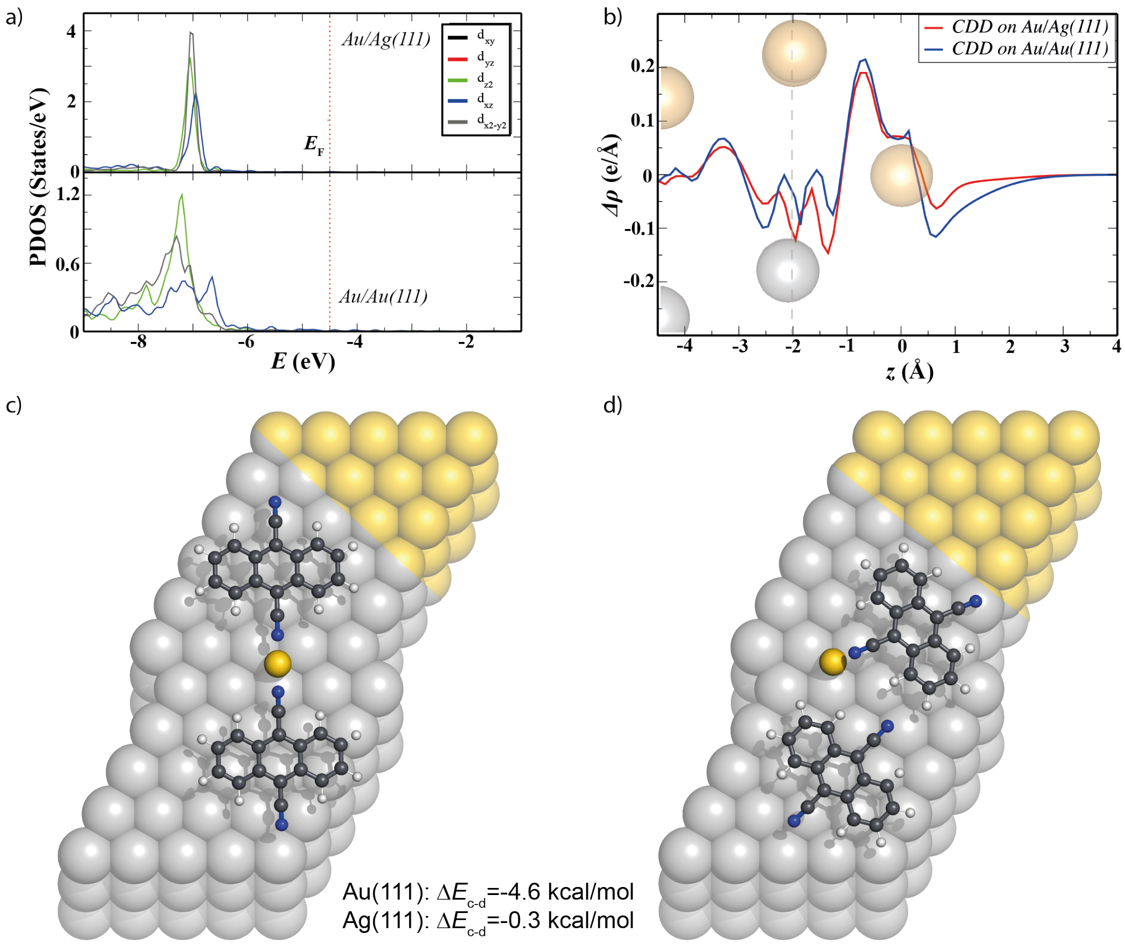


Figure S6: (a) Projected density of states (PDOS) onto Au 5d states for Au adatom on Ag(111) and on Au(111), as a function of energy, calculated via DFT (GGA-PBE). Energy broadening of the adatom Au 5d states on Au(111) is indicative of significant hybridization with the surface, while the sharp PDOS on Ag(111) indicates that the electronic character of Au on Ag(111) is close to that of an isolated neutral Au atom. (b) 1D projected charge density difference, $\Delta\rho$, for Au adatom on Au(111) (blue curve) and on Ag(111) (red curve), as a function of coordinate $z$ normal to the surface. Au adatom position corresponds to $z = 0$. Dashed vertical line indicates position of top-most layer of Ag(111) and Au(111). c), d) Ball-and-stick schematics of two different metal-organic complexes on Au(111) and Ag(111), consisting of 2 DCA molecules coordinated to an Au adatom via their nitrogen atoms. Total energy differences, $\Delta E$, between complexes in c) and d), on Au(111) and Ag(111), calculated by DFT (GGA-PBE).

We considered the total energy (calculated via DFT at the GGA-PBE level; see Methods) of different metal-organic complexes on both Au(111) and Ag(111) [Figure S6c), d)]. These complexes consisted of 2 DCA molecules coordinated to an Au adatom via their cyano N atoms, in different configurations.

On Au(111), the configuration where the Au adatom is coordinated to the cyano groups of the two DCA molecules in a linear geometry [Figure S6c)] is 4.6 kcal/mol more stable than the configuration where the Au adatom is coordinated to the cyano group of one DCA and interacts with the hydrogen atoms of the other [Figure S6d)]. On Ag(111), this difference is reduced to a negligible 0.3 kcal/mol. That is, different configurations of cyano-coordinated DCA-Au complexes with similar total energies might co-exist on Ag(111). In contrast, cyano-Au interactions dominate on Au(111). This provides an explanation for the difference between our present study and the previously observed honeycomb-kagome metal-organic framework on Au(111) where DCA and Au adatoms are coordinated via the DCA cyano groups.[18]

These different configurations of energetically similar, cyano-coordinated DCA-Au complexes on Ag(111) suggest that a dynamic equilibrium between different metal-organic phases could be present at room temperature. This dynamic equilibrium could then evolve irreversibly towards the experimentally observed DCA-Au-DCA dimers (via the regioselective C-H activation mechanism discussed in the main text and below).

# S8 C-H bond dissociation energies: QM/MM calculations

In Figure S7, we considered two different C-H bond dissociation mechanisms in a system composed of a single DCA molecule and a single Au adatom on Ag(111) (system 1 in main text): one involving the interaction between Au and the position A C-H bond [Figure S7b-d)]; the other involving the interaction between Au and the position B C-H bond [Figure

S7e-g)]. Note that the C-H bond dissociation enthalpies (BDE) for positions A and B in gas phase DCA are very similar [Figure S7a)]. The experimentally observed regioselectivity of the C-H bond cleavage therefore cannot be explained by differences in BDE. We performed QM/MM simulations (at $T = 0$ K first) to calculate the total energy differences, $\Delta E$, along these two reaction pathways, as an initial estimate of activation barriers. These calculations yielded similar energy differences between transition (TS) and initial (IS) states of 50.2 and 52.9 kcal/mol for positions A and positions B, respectively. This C-H bond dissociation mechanism mediated by a single Au adatom interacting with a single DCA molecule therefore also fails to explain the selectivity of the C-H scission at position A observed in experiments.

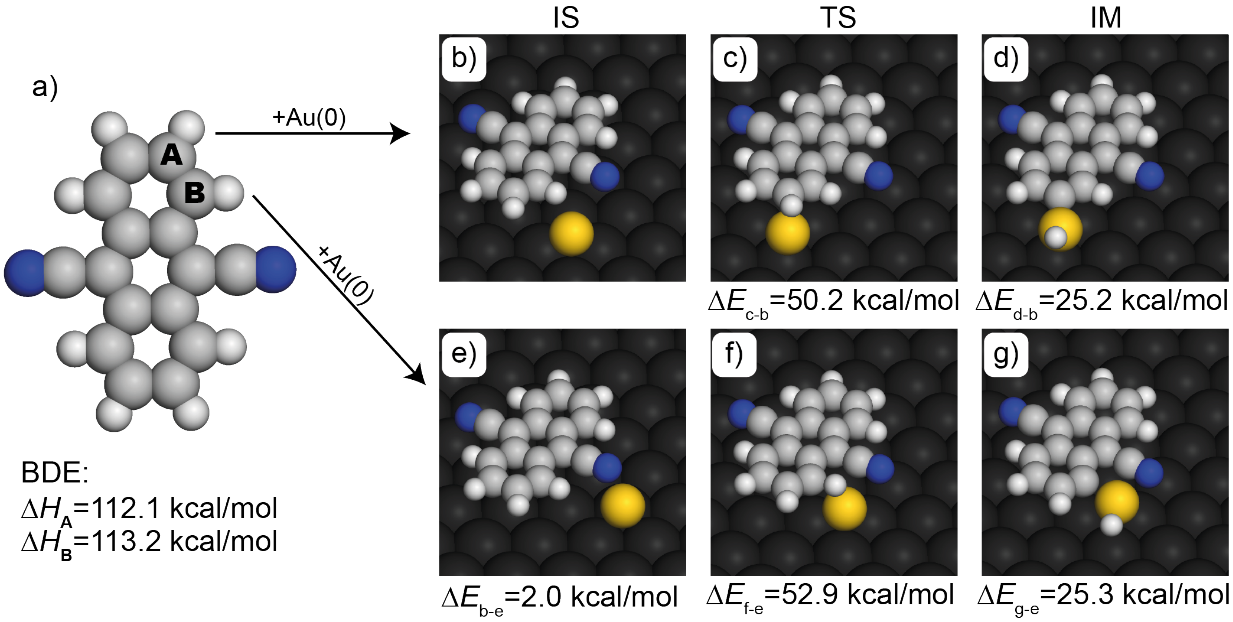


Figure S7: Different pathways for C-H bond cleavage in a single DCA molecule induced by a single Au adatom on Ag(111): QM/MM calculations at $T = 0$ K. a) Ball-and-stick structure of gas-phase DCA, with positions A and B C-H bond dissociation enthalpies (BDE), $\Delta H_{\mathrm{A,B}}$, calculated via DFT (see Methods). b) - g) Ball-and-stick models of initial (IS), transition (TS) and intermediate (IM) states along positions A (b - d) and B (e - g) C-H bond dissociation pathways, with total energy differences $\Delta E$ calculated via QM/MM simulations at $T = 0$ K.

We then performed QM/MM calculations at $T = 0$ K for similar C-H dissociation processes for a system composed of two DCA molecules and a single Au adatom on Ag(111) (Figure S8; system 2 in main text). Interestingly, these calculations show that C-H bond

dissociation pathways that involve a TS where DCA coordinates to Au via a metal-ligand bond at one of its cyano N atoms yield a substantially reduced energy difference $\Delta E$ between TS and IS (≈30 kcal/mol) for the C-H activation of an adjacent DCA molecule, for both positions A [Figure S8b), e)] and B [Figure S8c), f)]. While these calculations do not support the experimentally observed regioselectivity either, the lowering of these energy differences does suggest that a metal-organic cyano-Au motif may facilitate C-H bond cleaving.

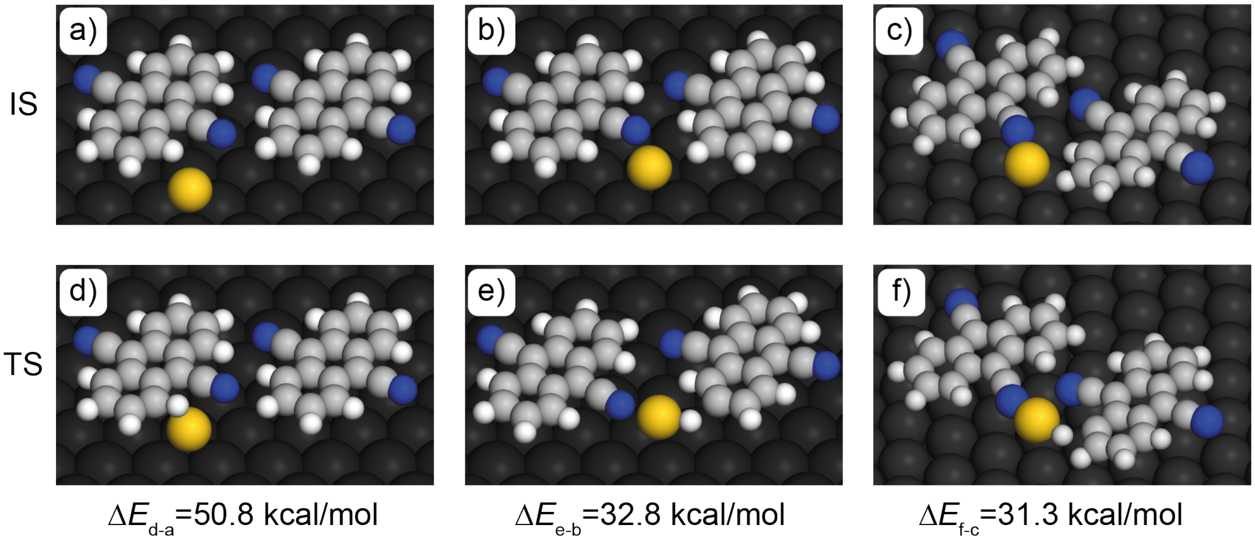


Figure S8: QM/MM calculated total energy differences, $\Delta E$, at $T = 0$ K between TS and IS for systems containing two DCA molecules and a single Au atom on Ag(111). A significant reduction in the energy difference is observed when a TS consisting of a metal-organic DCA-Au complex (with a N--Au coordination bond) is formed, for both positions A and B.

These findings motivated the QM/MM calculations at $T = 300$ K (i.e., close to our experimental conditions; see Methods) shown in the main text. These QM/MM calculations allowed us to determine the Gibbs free energy differences $\Delta G$ (and hence the activation barriers, defined as $\Delta G$ between transition and initial states) for the considered C-H bond dissociation pathways. That is, the total energy differences $\Delta E$ above and $\Delta G$ are strictly not identical, although they are related, with $\Delta E(T = 0)$ providing an initial estimate of $\Delta G$.

## S9 Orbital hybridization in reaction pathway

The QM/MM calculations reveal a significant lowering of the C-H dissociation barrier in DCA on Ag(111), when DCA interacts with a DCA--Au complex (in which Au forms a metal-organic coordination bond with a cyano N atoms). This interaction gives rise to an intermediate metal-organic H-Au--(N)DCA complex (with a linear H-Au--N motif) and to a DCA· radical (with a cleaved anthracene extremity C-H bond; Figure S8).

In the following, we focus on the electronic properties of the H-Au--(N)DCA intermediate, and present a hypothetical mechanism that explains the lowering of the DCA C-H bond activation barrier via such an intermediate. We calculated (via DFT at the B3LYP level; see Methods) the density of states (DOS) and projected DOS (PDOS) of three different isolated systems to analyze the nature of the bonding between Au and DCA in this intermediate: H-Au (Figure S9), Au--(N)DCA (Figure S10) and H-Au--(N)DCA (S11).

We first considered the DOS of H-Au (Figure S9). The total DOS reveals three molecular orbitals of hybrid Au and H character. Projecting the density of states of these three orbitals onto the Au atomic orbitals reveals they have predominantly $5d_{z2}$, 6s and $6p_z$ character as well as H 1s character. We identify these orbitals as bonding ($\sigma$), non-bonding (nb) and anti-bonding ($\sigma^*$) orbitals.

We then considered the DOS of a Au--(N)DCA system (Figure S10). In contrast to the findings for Au-H, the calculated DOS of this system reveals very little hybridization of Au states. Figure S10b) shows the PDOS onto Au atomic orbitals (solid lines) relative to PDOS for an isolated, neutral Au atom (dashed lines). All Au orbitals are shifted upwards in energy by the proximity to DCA, but their relative energies and appearance in the PDOS are fundamentally unchanged. This suggests negligible hybridization due to Au--N bonding, and no bonding or antibonding orbitals are formed. The interaction energy between Au and DCA in the complex is small ($\sim$4 kcal/mol), pointing to a weak interaction via polarization and electrostatics. Figure S10d) shows the charge density difference, which reveals a significant local polarization of the Au atom due to the proximity of the cyano group. This local

polarization causes intra-atomic charge redistribution within the Au atom. In particular, we observe electron accumulation in a ring surrounding the Au atom (green isosurface), balanced by electron depletion (pink) along the Au-cyano axis. Importantly, there is electron depletion on the outside of the Au atom, in the direction from which a H atom could approach to form the intermediate DCA(H)-Au--(N)DCA complex (see $IM_{2A}$ in main text and below). The depleted density on the Au adatom reduces the Pauli repulsion between the Au and H atoms. This facilitates the formation of a chemical bond between Au and H.

Lastly, we considered the DOS of a H-Au--(N)DCA system (Figure S11). In Figure S11 we find that the $\sigma$, nb and $\sigma^*$ orbitals seen for Au-H are preserved for this system. This can be clearly seen in the comparison between Au-H and H-Au--(N)DCA DOS shown in Figure S12. In the case of H-Au--(N)DCA, however, $\sigma$ and $\sigma^*$ orbitals undergo further hybridization with the N orbitals of DCA which results in further splitting of the $\sigma^*$ orbital. While this Au-N hybridization is still relatively minor and does not support the claim of a dative bond, the interaction energy between Au and N increases significantly (by $\sim$22 kcal/mol) for this system, with a corresponding reduction in Au--N distance of $\sim$0.5 Å, relative to the Au--(N)DCA system.

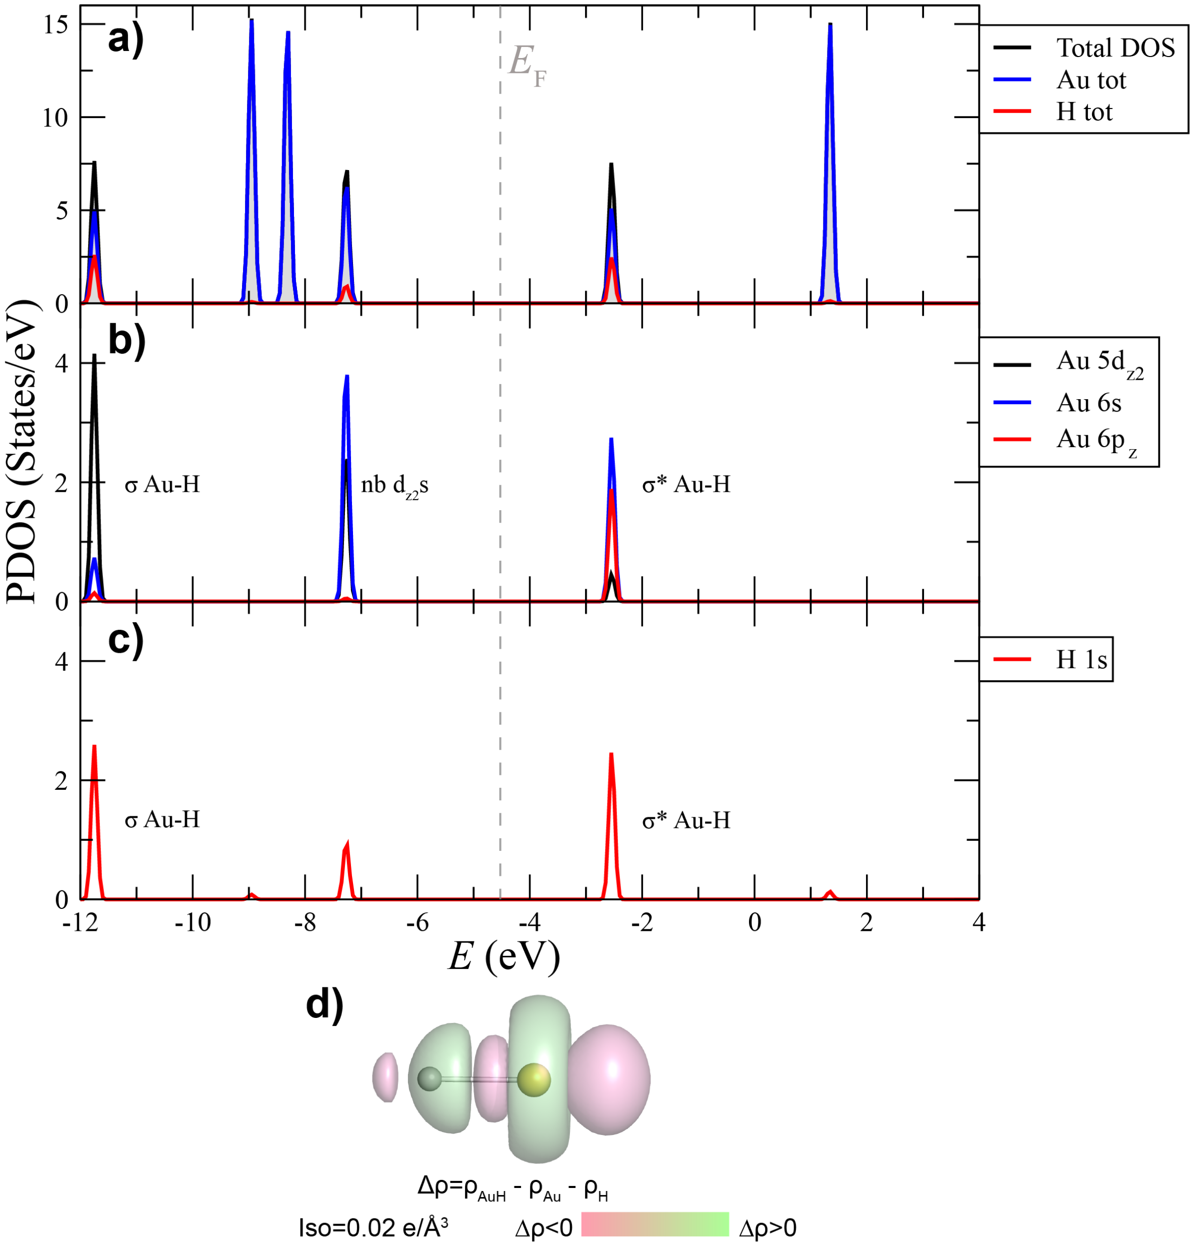


Figure S9: Density of states (DOS) and orbital character of isolated Au-H system, calculated via DFT (B3LYP). (a) Total DOS (black curve with gray filling) and projected DOS (PDOS; blue: onto Au states; red: onto H states), as a function of energy. (b) PDOS projected onto Au 5d$_{z2}$, Au 6s and Au 6p$_z$ orbitals, as a function of energy. (c) PDOS onto H 1s states. Au-H system bonding ($\sigma$), antibonding ($\sigma$) orbitals, and non-bonding (nb) d$_{z2}$s hybrid orbital are indicated. (d) Electron density difference $\Delta\rho$ between Au-H system, and neutral isolated Au(0) atom and neutral isolated H atom.

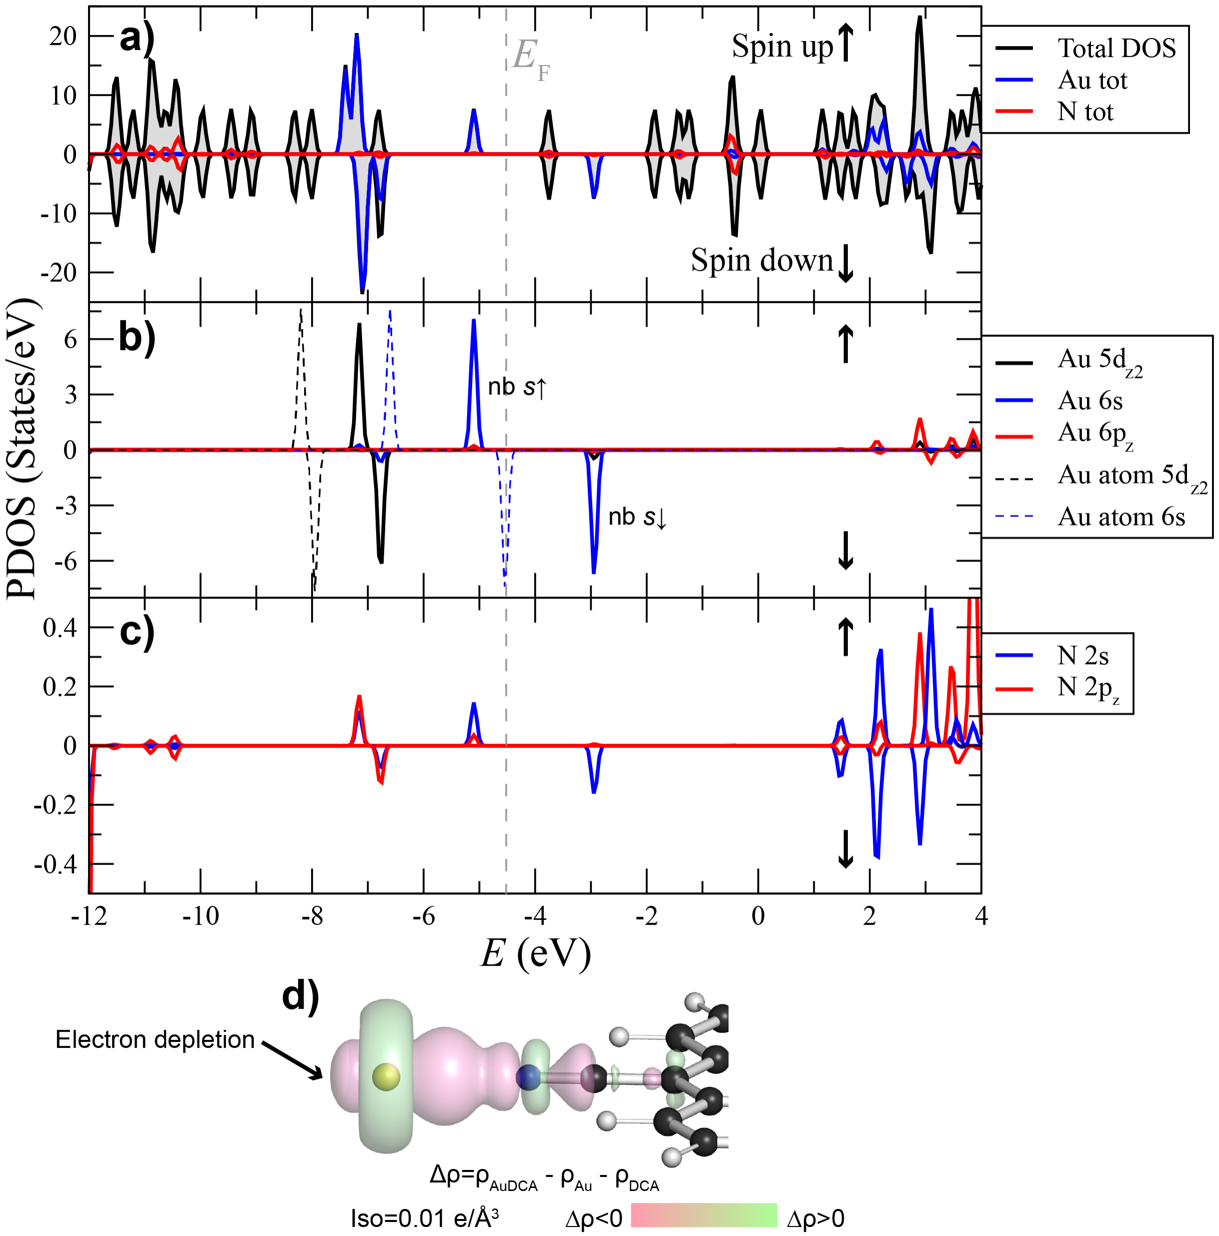


Figure S10: Density of states (DOS) and orbital character of Au--(N)DCA system, calculated via DFT (B3LYP). (a) Total DOS (black with gray filling) and projected DOS (PDOS; blue: onto Au states; red: onto states of N atom coordinated with Au), as a function of energy. (b) PDOS, projected onto Au $5d_{z2}$, 6s and $6p_z$ orbitals, as function of energy. Dashed curves correspond to an isolated neutral Au atom, for comparison. (c) PDOS onto N 2s and $2p_z$ orbitals. (d) Electron density difference $\Delta\rho$ between Au--(N)DCA, and neutral isolated Au(0) atom and neutral isolated DCA. Spin degeneracy lifting shown for this figure as the net electronic structure is open-shell (not the case for other figures in this section).

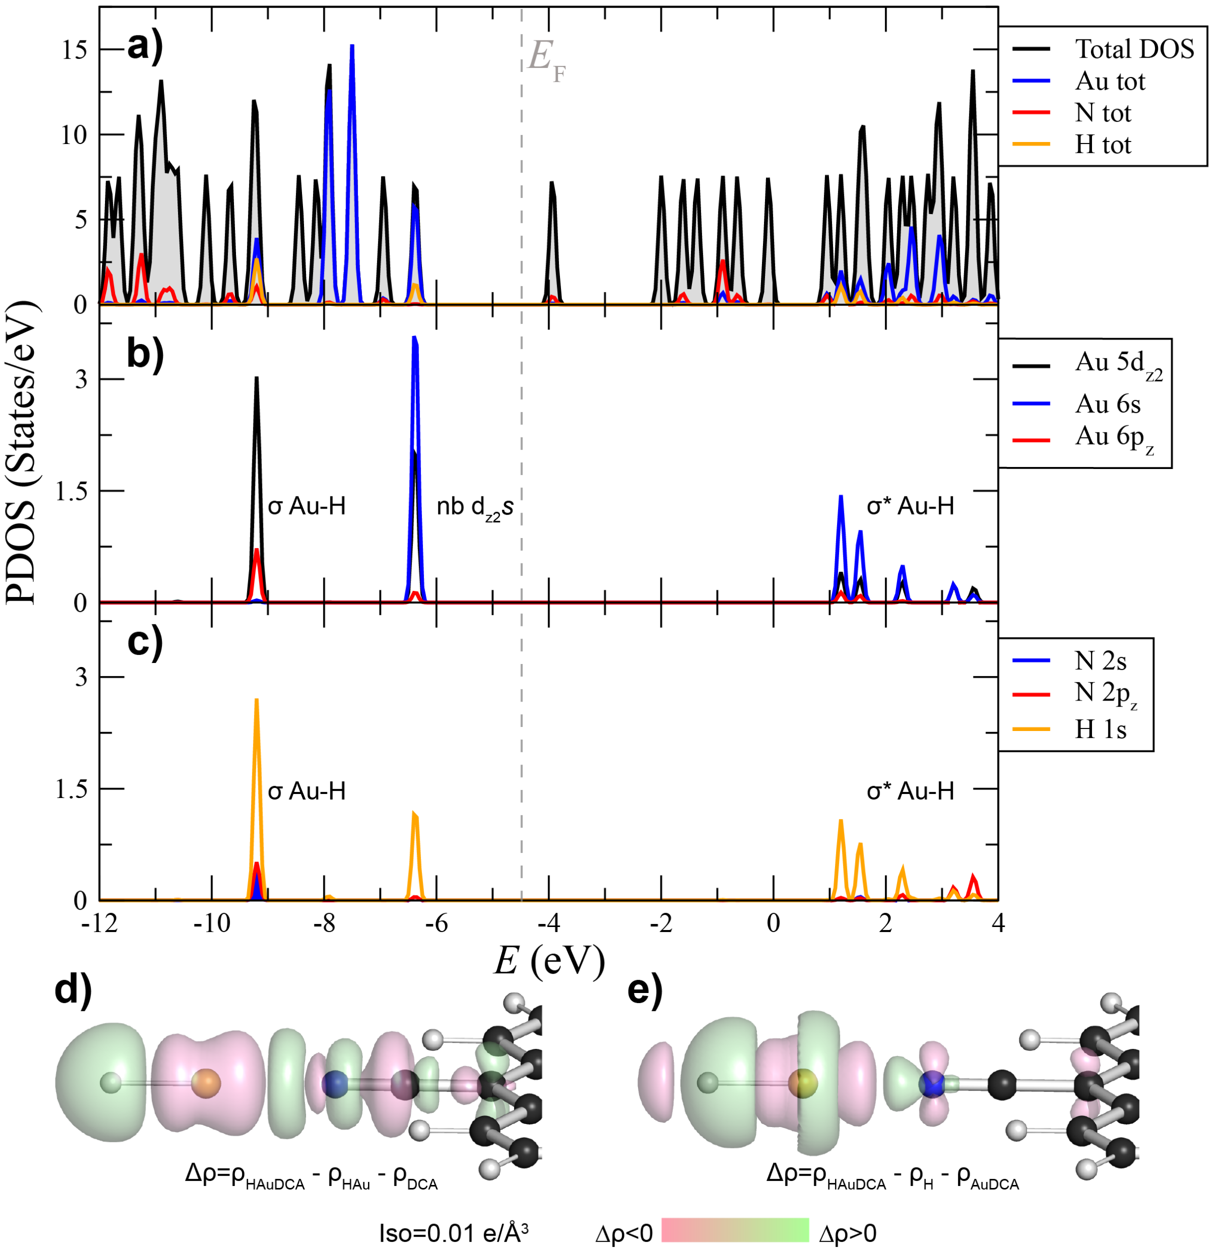


Figure S11: Density of states (DOS) and orbital character of H-Au--(N)DCA system, calculated via DFT (B3LYP). (a) Total DOS (black with gray filling) and projected DOS (PDOS; blue: onto Au states; red: onto states of N atom coordinated with Au; orange: onto states of H atom coordinated with Au), as a function of energy. (b) PDOS, projected onto Au $5d_{z2}$, 6s and $6p_z$ orbitals, as function of energy. (c) PDOS onto N 2s and $2p_z$ orbitals, and onto H 1s orbital. We identify $\sigma$ bonding (hybridization between Au $5d_{z2}$, Au $6p_z$ and H 1s dominantly with some N s and $p_z$ character) and $\sigma^*$ antibonding (mainly Au 6s - H 1s - N $p_z$ hybridization) orbitals, as well as a hybrid non-bonding (nb) orbital with Au 6s, Au $d_{z2}$ and H 1s character. (d-e) Electron density difference $\Delta\rho$ between H-Au--(N)DCA and system composed of H-Au and isolated DCA (d), and between H-Au--(N)DCA and system composed of isolated neutral H and Au--DCA (e).

The electrostatic potentials in Figure S12c-d) show a partial positive charge $\delta^{+}$ at the Au extremity of the H-Au system, and a partial negative charge $\delta^{-}$ at the DCA N atom. We claim that the formation of the $\sigma$, nb and $\sigma^{*}$ orbitals due to H-Au hybridization reduces the electrostatic repulsion between the occupied Au 5d orbitals and lone electron-pair of the DCA N atom; this stabilizes the complex.

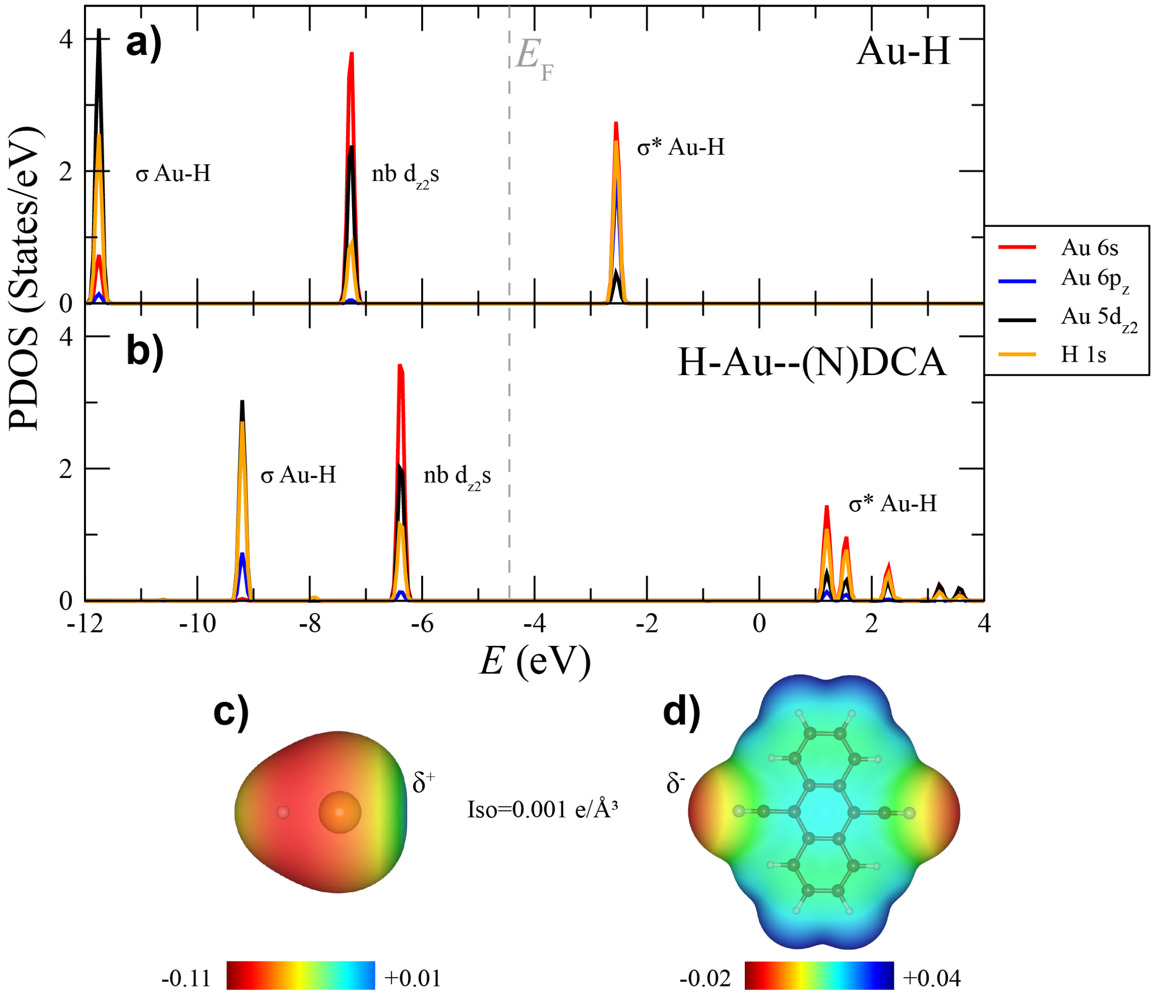


Figure S12: Comparison of PDOS of Au-H and H-Au--(N)DCA systems (projections onto Au $5d_{z2}$, 6s and $6p_z$, and H 1s orbitals). (a) PDOS of Au-H system as a function of energy. (b) PDOS of H-Au--(N)DCA system as a function of energy. (c), (d) Isosurface (0.001 $e$/ Å $^{3}$) of electrostatic potential, $\Phi_{\text{el}}$ (calculated from the DFT electron density), for Au-H (c) and isolated DCA (d) systems, showing electrostatic attraction between Au and DCA N atom.

The hybridization between Au 5d$_{z2}$, Au 6s and Au 6p$_z$ orbitals in H-Au and H-Au--(N)DCA is similar to that observed in linear Au(I) complexes, where fully occupied Au 5d and empty 6s orbitals are nearly degenerate.[19] In these Au(I) complexes, 5d$_{z2}$ and 6s orbitals hybridize as illustrated in Figure S13a). The $\Psi_1 = d_{z2} + s$ orbital is fully occupied and thus remains non-bonding (nb). Its torus shape lowers the electrostatic repulsion with nearby ligands (often facilitating linear Au complexes with a coordination number of 2). The $\Psi_2 = d_{z2} - s$ orbital is empty and can further hybridize with the Au 6p$_z$ orbital, forming two hybrid Au 5d - Au 6s - Au 6p acceptor orbitals $\Psi_2 \pm p_z$ as shown in Figure S13b).

In the case of H-Au--(N)DCA above, we only observed hybridization between Au 5d and Au 6s orbitals. The resulting $\Psi_1$ orbital is non-bonding, while $\Psi_2$ forms a $\sigma$ bond with H 1s. There is no indication of further hybridization with Au 6p orbitals nor of dative bonding between N and Au. After the formation of the covalent H-Au bond, the electron density related to the $\Psi_2$ orbital is similar to that of hydrogen, thus lowering its repulsion with the lone electron pair of nitrogen.

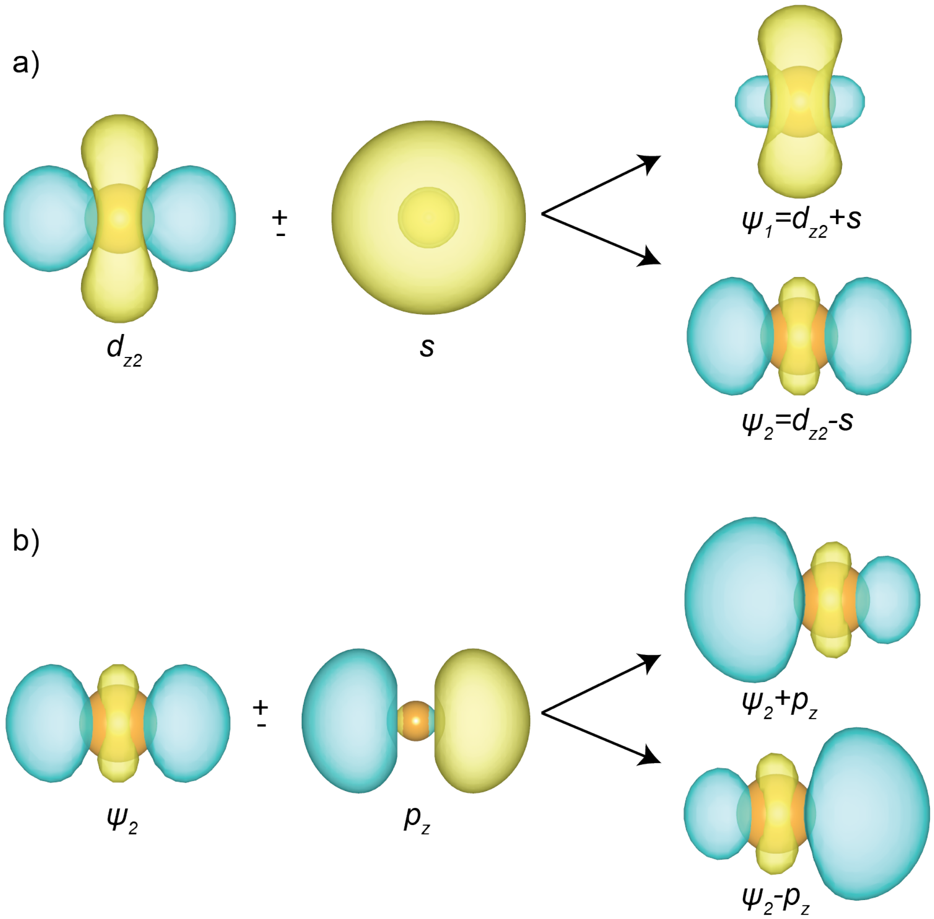


Figure S13: Hybridization of Au 5d$_{z2}$, Au 6s and Au 6p$_z$ states. (a) Schematic of Au 5d$_{z2}$ - Au 6s hybridization, forming orbitals $\Psi_1$ and $\Psi_2$. Upon Au-H bonding, both these orbitals can hybridize with H 1s. $\Psi_1$ gives rise to the non-bonding orbital present in Figures S9-S12 whereas $\Psi_2$ gives rise to $\sigma$ bonding and $\sigma^*$ anti-bonding orbitals in H-Au and H-Au--(N)DCA. (b) Further hybridization between $\Psi_2$ and Au 6p$_z$ orbital yields two equivalent linear orbitals $\Psi_2 \pm p_z$, as observed in coordination chemistry of Au(I).

We claim that when the system composed of 2 DCA molecules and a Au adatom on Ag(111) is in the initial state IS$_{2A}$ [consisting of Au--(N)DCA and another DCA; see Figure 5c) in main text], a position A C-H stretching mode can facilitate the cleavage of the C-H bond closest to Au. We claim that the stabilization of the Au--N interaction as the system progressively transitions from Au--(N)DCA to H-Au--(N)DCA is at the basis of the low C-H activation barrier observed.

## S10 Tentative pathway to organometallic dimers

Figure S14 highlights the geometry at the edge of a self-assembled DCA-only domain. The arrangement of DCA molecules at such an edge is similar to that in initial states $IS_{2A}$ and $IS_{2B}$ in Figure 5c), d) of main text (omitting Au atom).

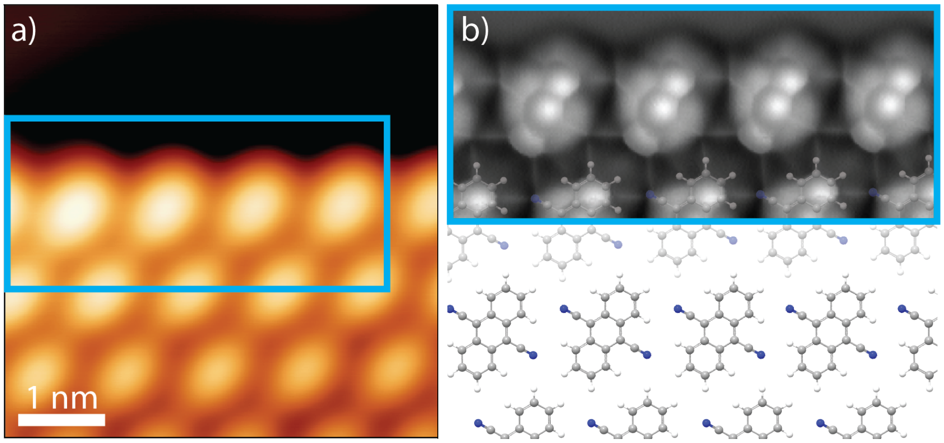


Figure S14: a) Constant-current STM image showing the edge of a self-assembled DCA-only domain on Ag(111) ($V_b = -50$ mV, $I_t = 50$ pA). b) NcAFM image acquired at the blue box in a) (acquired at a height 30 pm closer to the sample than the setpoint $V_b = 15$ mV, $I_t = 100$ pA) with overlaid ball-and-stick model of self-assembly . These images highlight the geometry at the edge of the DCA film.

We observed self-assembled DCA+Au domains composed of organometallic DCA-Au-DCA dimers both via co-deposition of Au and DCA, and via sequential deposition of DCA and then Au. This shows that the DCA-Au-DCA units can form after the DCA-only self-assembly. The supramolecular DCA-only domains are robust, with each DCA molecule within the domain participating in eight non-covalent H–N bonds with neighboring molecules, with each bond having an interaction energy of ~7.1 kcal/mol based on DFT calculations (B3LYP level). We suggest that the self-assembled DCA-only domains may facilitate the Au-induced C-H bond cleavage, with Au adatoms interacting with cyano groups at the edge of the DCA-only domains. In the following, we propose a tentative reaction pathway from self-assembled DCA-only domains to the observed organometallic DCA-Au-DCA units; see Figure S15. Figure S15a) shows an Au adatom interacting with a cyano N

atom of an edge DCA molecule, forming the initial state $IS_{2A}$ of Figure 5c) in the main text. This then can lead to the cleavage of the position A C-H bond of an adjacent edge DCA molecule [Figure S15b)], resulting in an intermediate state similar to that of $IM_{2A}$ [Figure 5c) of main text] with a DCA· radical. Based on DFT (GGA-PBE) calculations, we suggest that, subsequently, the hydrogen atom is likely to prefer bonding directly to Ag(111) than to the Au adatom on Ag(111) - as the former case is ∼4.5 kcal/mol more stable. This would allow the DCA· radical to then further react with a Au adatom [Figure S15c), d)], and finally with another DCA· radical, forming the organometallic DCA-Au-DCA dimer that we observed experimentally. We also suggest that non-covalent N–H bonds between neighboring DCA-Au-DCA within a DCA+Au domain contribute to the stabilization of this phase (which are not accounted for in simulations shown in Figure 5).

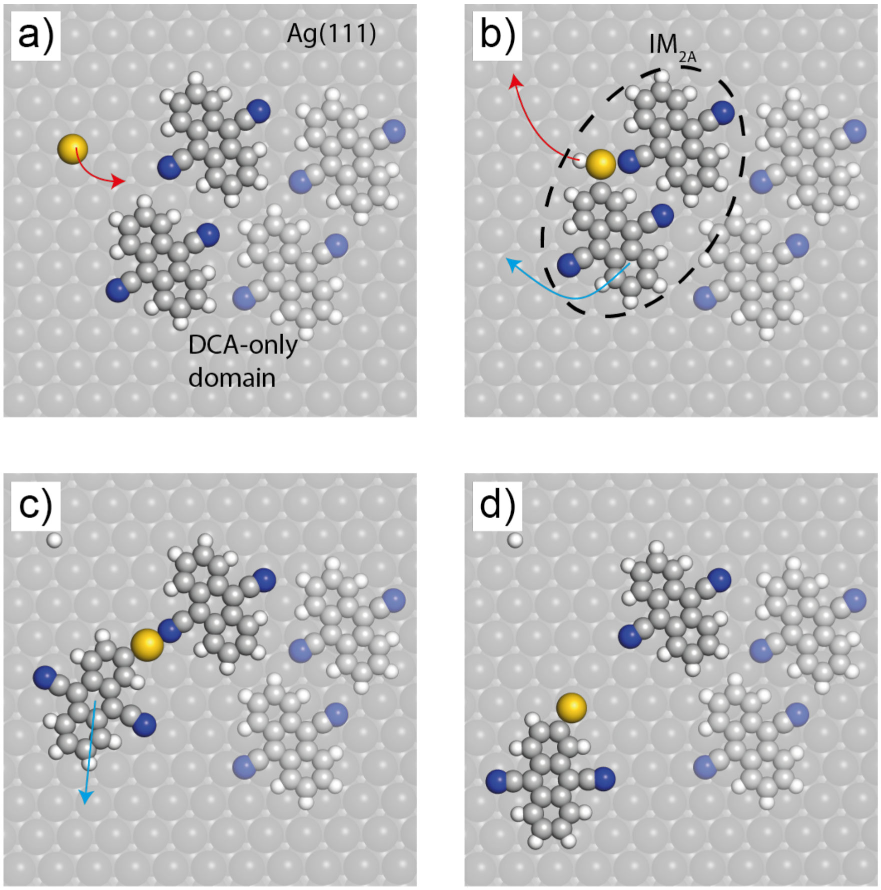


Figure S15: Ball-and-stick schematic of C-H bond cleavage mechanism at DCA-only domain edge. (a) Au adatom interacts with cyano N atom of DCA molecule at DCA-only domain edge, forming a Au--(N)DCA metal-organic complex and the initial state $IS_{2A}$ [Figure 5c) of main text]. (b) Metal-organic Au--(N)DCA complex at DCA-only domain edge interacts with adjacent DCA molecule. This leads to cleavage of position A C-H bond in the adjacent DCA molecule, resulting in the formation of transition ($TS_{2A}$) and intermediate ($IM_{2A}$) states [Figure 5c) of main text] composed of a metal-organic H-Au--(N)DCA complex and a DCA· radical. Blue arrow represents rotation of DCA· radical to accommodate linear H-Au--(N)DCA complex in $IM_{2A}$. Red arrow illustrates subsequent migration of H atom from Au adatom onto Ag(111) surface. (c) Radical DCA· molecule can then interact with Au adatom and form a C-Au covalent bond. Blue arrow represents dissociation of Au--N bond and detachment of DCA(C)-Au complex from DCA-only domain. (d) DCA(C)-Au complex can then diffuse and interact with another DCA· radical, forming an organometallic DCA-Au-DCA unit.

# S11 Second C-H bond activation

We considered the possibility of a second position A C-H bond cleavage occurring at the anthracene end opposite to Au in a DCA-Au-DCA dimer. Figure S16 shows transition states (TS) of a system composed of an organometallic DCA-Au-DCA unit, an extra DCA molecule and an extra Au adatom on Ag(111). We performed QM/MM calculations (at $T = 0$ K) of total energy differences $\Delta E$ (i.e., estimates of activation barriers) between TS and IS for C-H bond cleaving in a DCA-Au-DCA dimer, at position A opposite to the Au center, mediated by a metal-organic Au--(N)DCA complex [Figure S16a)]. We obtained $\Delta E_{\text{TS-IS}} \approx 63.0$ kcal/mol. This energy difference is ∼twice that estimated for a position A C-H bond cleavage in an isolated DCA, mediated by a Au--(N)DCA-Au-DCA complex [$\sim$ 31.8 kcal; Figure S16b)]. This suggests that the formation of 1D -[Au-DCA-Au-DCA]- organometallic chains is not energetically favorable, and that the DCA-Au-DCA dimers are stable discrete units, consistent with our experimental observations.

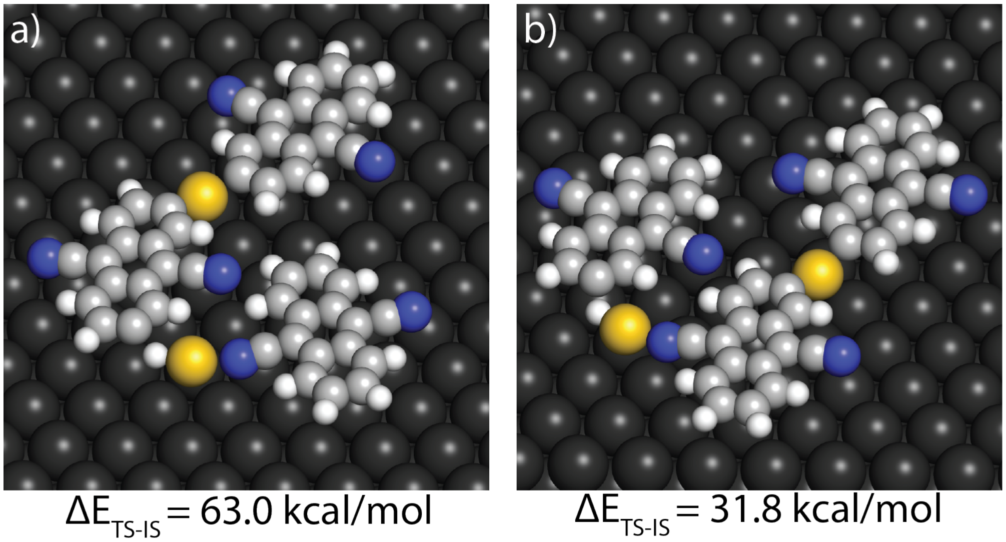


Figure S16: QM/MM calculated total energy differences at $T = 0$ K, $\Delta E$, between transition (TS) and initial (IS) states of systems comprised of an organometallic DCA-Au-DCA unit, an extra DCA molecule and an extra Au adatom on Ag(111). (a) Energy difference between TS and IS for cleavage of position A C-H bond in DCA-Au-DCA dimer opposite to Au center, mediated by Au--(N)DCA complex, is 63.0 kcal/mol. (b) Energy difference between TS and IS position A C-H bond cleavage in isolated DCA, mediated by Au–(N)DCA-Au-DCA complex, is significantly lower, 31.8 kcal/mol. This suggests that 1D -[Au-DCA-Au-DCA]-organometallic polymerization is not favorable, consistent with the experimental observation of discrete DCA-Au-DCA dimers.

# References

(1) Frisch, M. J. et al. Gaussian16 Revision C.01. 2016.

(2) Chai, J.-D.; Head-Gordon, M. Long-range corrected hybrid density functionals with damped atom–atom dispersion corrections. *Phys. Chem. Chem. Phys.* **2008**, *10*, 6615–6620.

(3) Weigend, F.; Ahlrichs, R. Balanced basis sets of split valence, triple zeta valence and quadruple zeta valence quality for H to Rn: Design and assessment of accuracy. *Phys. Chem. Chem. Phys.* **2005**, *7*, 3297–3305.

(4) Blum, V.; Gehrke, R.; Hanke, F.; Havu, P.; Havu, V.; Ren, X.; Reuter, K.; Scheffler, M.

Ab initio molecular simulations with numeric atom-centered orbitals. *Computer Physics Communications* **2009**, *180*, 2175–2196.

(5) Lee, C.; Yang, W.; Parr, R. G. Development of the Colle-Salvetti correlation-energy formula into a functional of the electron density. *Phys. Rev. B* **1988**, *37*, 785–789.

(6) Tkatchenko, A.; Scheffler, M. Accurate Molecular Van Der Waals Interactions from Ground-State Electron Density and Free-Atom Reference Data. *Phys. Rev. Lett.* **2009**, *102*, 073005.

(7) Perdew, J. P.; Burke, K.; Ernzerhof, M. Generalized Gradient Approximation Made Simple. *Phys. Rev. Lett.* **1996**, *77*, 3865–3868.

(8) Case, D. A. et al. Amber 2020. 2020.

(9) Lewis, J. P.; Jelínek, P.; Ortega, J.; Demkov, A. A.; Trabada, D. G.; Haycock, B.; Wang, H.; Adams, G.; Tomfohr, J. K.; Abad, E.; Wang, H.; Drabold, D. A. Advances and applications in the FIREBALL ab initio tight-binding molecular-dynamics formalism. *physica status solidi (b)* **2011**, *248*, 1989–2007.

(10) Becke, A. D. Density-functional exchange-energy approximation with correct asymptotic behavior. *Phys. Rev. A* **1988**, *38*, 3098–3100.

(11) Grimme, S.; Ehrlich, S.; Goerigk, L. Effect of the damping function in dispersion corrected density functional theory. *Journal of Computational Chemistry* **2011**, *32*, 1456–1465.

(12) Basanta, M. A.; Dappe, Y. J.; Jelínek, P.; Ortega, J. Optimized atomic-like orbitals for first-principles tight-binding molecular dynamics. *Computational Materials Science* **2007**, *39*, 759–766.

(13) Becke, A. D. Density-functional thermochemistry. III. The role of exact exchange. *J. Chem. Phys.* **1993**, *98*, 5648–5652.

(14) Vosko, S. H.; Wilk, L.; Nusair, M. Accurate spin-dependent electron liquid correlation energies for local spin density calculations: a critical analysis. *Can. J. Phys.* **1980**, *58*, 1200–1211.

(15) Liu, X.; Matej, A.; Kratky, T.; Mendieta-Moreno, J. I.; Günther, S.; Mutombo, P.; Decurtins, S.; Aschauer, U.; Repp, J.; Jelinek, P.; Liu, S.-X.; Patera, L. L. Exploiting Cooperative Catalysis for the On-Surface Synthesis of Linear Heteroaromatic Polymers via Selective C–H Activation. *Angewandte Chemie International Edition* **2022**, *61*, e202112798.

(16) Hapala, P.; Kichin, G.; Wagner, C.; Tautz, F. S.; Temirov, R.; Jelínek, P. Mechanism of high-resolution STM/AFM imaging with functionalized tips. *Phys. Rev. B* **2014**, *90*, 085421.

(17) Kumar, D.; Krull, C.; Yin, Y.; Medhekar, N. V.; Schiffrin, A. Electric Field Control of Molecular Charge State in a Single-Component 2D Organic Nanoarray. *ACS Nano* **2019**, *13*, 11882–11890.

(18) Yan, L.; Pohjavirta, I.; Alldritt, B.; Liljeroth, P. On-Surface Assembly of Au-Dicyanoanthracene Coordination Structures on Au(111). *ChemPhysChem* **2019**, *20*, 2297–2300.

(19) Orgel, L. E. 843. Stereochemistry of metals of the B sub-groups. Part I. Ions with filled d-electron shells. *J. Chem. Soc.* **1958**, 4186–4190.
